# Supplementary material for: Observation of nonreciprocal magnon Hanle effect
Source: arXiv:2209.09040 source file (2022-09-19)
Supplement: Supplementary file 1 [file SM_nonrec_Hanle.pdf]

# Supplemental Material: Observation of nonreciprocal magnon Hanle effect

Janine Gückelhorn,[1,2,*] Sebastián de-la-Peña,[3] Matthias Grammer,[1,2]
Monika Scheufele,[1,2] Matthias Opel,[1] Stephan Geprägs,[1] Juan Carlos Cuevas,[3]
Rudolf Gross,[1,2,4] Hans Huebl,[1,2,4] Akashdeep Kamra,[3,†] and Matthias Althammer[1,2,‡]

[1] *Walther-Meißner-Institut, Bayerische Akademie der Wissenschaften, D-85748 Garching, Germany*

[2] *Physik-Department, Technische Universität München, D-85748 Garching, Germany*

[3] *Condensed Matter Physics Center (IFIMAC) and Departamento de Física Teórica de la Materia Condensada, Universidad Autónoma de Madrid, E-28049 Madrid, Spain*

[4] *Munich Center for Quantum Science and Technology (MCQST), D-80799 München, Germany*

(Dated: September 16, 2022)

* janine.gueckelhorn@wmi.badw.de

† akashdeep.kamra@uam.es

‡ matthias.althammer@wmi.badw.de

## I. HEMATITE FILMS AND MAGNETOMETRY MEASUREMENTS

The 89 nm and 19 nm thin, single crystalline (0001)-oriented hematite ($\alpha - Fe_2O_3$) films investigted in this study were grown via pulsed laser deposition on (0001)-oriented sapphire ($Al_2O_3$) substrates. For the deposition in oxygen atmosphere, a substrate temperature of 320 °C, an oxygen pressure of 25 µbar, a laser fluence at the target of 2.5 J/cm$^2$ and a laser repetition rate of 2 Hz were used. To reduce oxygen vacancies, a RF-atom source was used to inject atomic oxygen into the chamber.

Hematite exhibits a Néel temperature of $T_N = 953$ K in bulk crystals and undergoes a spin reorientation, the Morin transition, at $T_M = 263$ K [S1]. This transition is based on a sign change of the uniaxial magnetic anisotropy, resulting in a transition from a magnetic [0001] easy-axis below $T_M$ to a magnetic easy (0001)-plane above $T_M$. To determine the Morin transition temperature in our thin films, we performed SQUID (superconducting

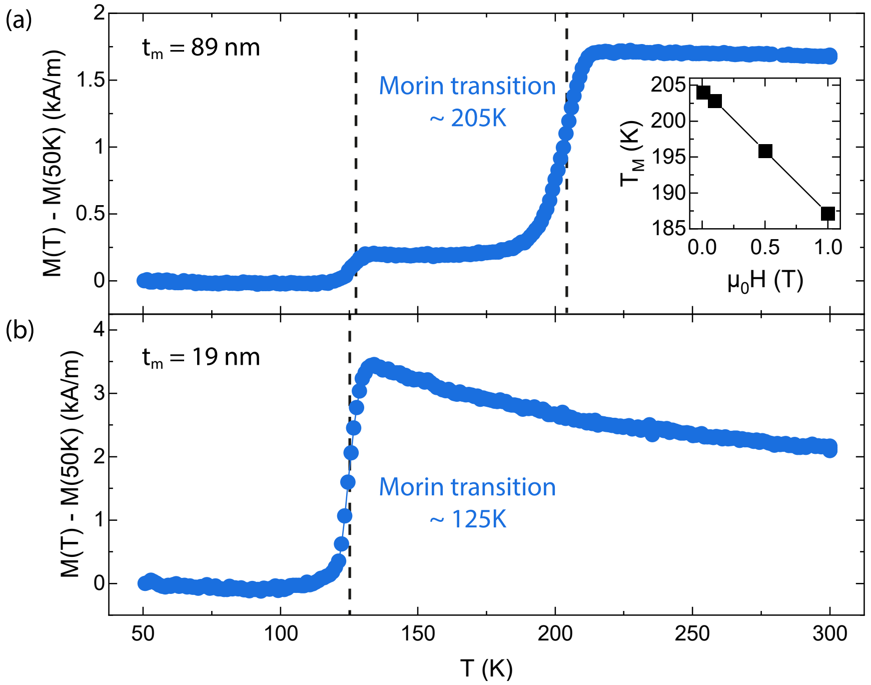


FIG. S1. In-plane magnetization versus temperature curves from 50 to 300 K at 100 mT obtained by SQUID magnetometry in zero field cooling (ZFC) configuration for the (a) $t_m = 89$ nm and (b) $t_m = 19$ nm thick thin film. In both cases, we can unambiguously identify the Morin transition. The inset in panel (a) shows the magnetic field dependence of the Morin transition temperature $T_M$.

quantum interference device) magnetometry measurements. The obtained magnetization $M$ is shown as a function of the temperature in Fig. S1 for an in-plane magnetic field of 100 mT in zero field cooling (ZFC) configuration. Note that a temperature independent, linear in magnetic field (diamagnetic) background stemming from the $Al_2O_3$ substrate was subtracted from the data. For the $t_m = 89\,\mathrm{nm}$ thick film in panel (a), we find a Morin transition at $T_M = 205\,\mathrm{K}$, while we obtain $T_M = 125\,\mathrm{K}$ for the thinner film shown in panel (b), both values being smaller than in bulk crystals. The additional transition around 125 K of the $t_m = 89\,\mathrm{nm}$ thick thin film suggests two different magnetic phases most probably due to a strained $\alpha - Fe_2O_3$ layer close to the interface to the $Al_2O_3$ substrate. The inset in Fig. S1(a) shows the magnetic field dependence of $T_M$. We find a decreasing Morin transition temperature with increasing magnetic field magnitude.

## II. ALL-ELECTRICAL MAGNON TRANSPORT MEASUREMENTS

To allow for an all-electrical generation and detection of pure spin currents, we use electron beam lithography to pattern two-strip (electrode) structures with varying center-to-center distances $d$ on top of the hematite films and deposit *ex-situ* polycrystalline 5 nm thick Pt by magnetron sputtering and a subsequent lift-off. In a further patterning step, Al leads and bondpads (50 nm thickness) were deposited to connect the device electrically. The Pt strip width is kept constant at $w_l = w_r = 500\,\mathrm{nm}$ and the strips have a length of $l = 100\,\mu\mathrm{m}$.

For the two-strip structure experiments (see Fig. 2(a) in the main text), we utilize the DC-detection technique. Here, a DC charge current $I^{\mathrm{inj}} = 500\,\mu\mathrm{A}$ is applied to the first Pt electrode using a Keithley 2400 Sourcemeter. A Keithley 2182 Nanovoltmeter is used to detect the magnon transport signal at the second electrode. Applying a current reversal technique, we can define the voltage due to SHE-induced magnons transported between the two electrodes as

$$V_{\mathrm{SHE}}^{\mathrm{det}} = \frac{1}{2}\left[V^{\mathrm{det}}\left(I^{\mathrm{inj}}\right) - V^{\mathrm{det}}\left(-I^{\mathrm{inj}}\right)\right] \ . \tag{S1}$$

From this we then calculate $R^{\mathrm{el}} = V_{\mathrm{SHE}}^{\mathrm{det}}/I^{\mathrm{inj}}$. All measurements are conducted above the Morin transition temperature, i.e. our samples feature an easy-plane phase. The measurements for the $t_m = 89\,\mathrm{nm}$ thick film are performed at $T = 250\,\mathrm{K}$, the ones for the $t_m = 19\,\mathrm{nm}$ thin film at $T = 200\,\mathrm{K}$.

## III. NON-RECIPROCAL MAGNON TRANSPORT IN A THIN HEMATITE FILM

In this section, we demonstrate that the antisymmetric signal contribution is also present in thin hematite films, where the contribution of low-energy magnons can be neglected [S2]. To this end, we investigate a 19 nm thin $\alpha-Fe_2O_3$ film with similar structures on top as for the thicker film depicted in Fig. 2(a) in the main text. Here, we perform angle-dependent measurements on a structure with a center-to-center distance $d = 0.75\,\mu m$. Fig. S2(a) shows the magnon spin signal as a function of the magnetic field orientation $\varphi$ with the same fixed magnitudes $\mu_0 H$ as for the thicker sample at a temperature of 200 K. Since the Hanle peak is shifted towards higher magnetic field values for thinner hematite layers [S2, S3], we measured at a slightly lower temperature to counteract this effect and have a sufficient high magnon spin signal at the same time [S3]. Similar to the main text, the filled dots correspond to magnons transported from the left to the right electrode, while the open circles correspond to the reversed measurement scheme or backwards propagating magnons. For $\mu_0 H = 5\,T$ and 6 T the angle-dependent magnon spin signal exhibits a very similar behavior for the forward ($R^{el}(+d)$) and the backward ($R^{el}(-d)$) propagation direction, while for $\mu_0 H = 7\,T$ we observe a clear difference, especially at $\varphi = 90°$ and 270°, when $\boldsymbol{H} \perp \boldsymbol{n}$. To investigate this behavior in more detail, we plot the symmetric signal $R^{el}_{sym} = (R^{el}(+d) + R^{el}(-d))/2$ in Fig. S2(b) and the antisymmetric signal of the two measurement configurations $R^{el}_{asym} = (R^{el}(+d) - R^{el}(-d))/2$ in Fig. S2(c). The symmetric signal $R^{el}_{sym}$ in panel (b) contains only the inversion-symmetric part, i.e. no differences in pseudofields $\boldsymbol{\omega}$ for the two propagation directions and $\delta\omega = 0$. We observe the expected $\sin^2(\varphi)$ dependence with an amplitude $\Delta R^{el}_{sym}$ as indicated by the solid lines in Fig. S2(b). Analog to the main text, the nonreciprocal signal in Fig. S2(c) can be described by a $\Delta R^{el}_{asym} \sin^3(\varphi)$ dependence (solid lines), where $\Delta R^{el}_{asym}$ quantifies the amplitude of the antisymmetric signal contribution. We clearly observe this behavior for $\mu_0 H = 7\,T$, where $\Delta R^{el}_{asym} = -30\,\mu\Omega$ at $\varphi = 90°$ and exhibits the same value, however with an inverse sign, for $\varphi = 270°$. This sign convention resembles the angle-dependence of the thicker hematite layer measured at $\mu_0 H = 5\,T$. For $\mu_0 H = 6\,T$ the signs of this effect remains the same, however the magnitude is significantly decreased, while it vanishes for $\mu_0 H = 5\,T$. This is in contrast to our results for the thicker hematite film, where we observed a sign change at $\varphi = 90°$ and 270° when we increased the magnetic field magnitude from 5 T to 7 T.

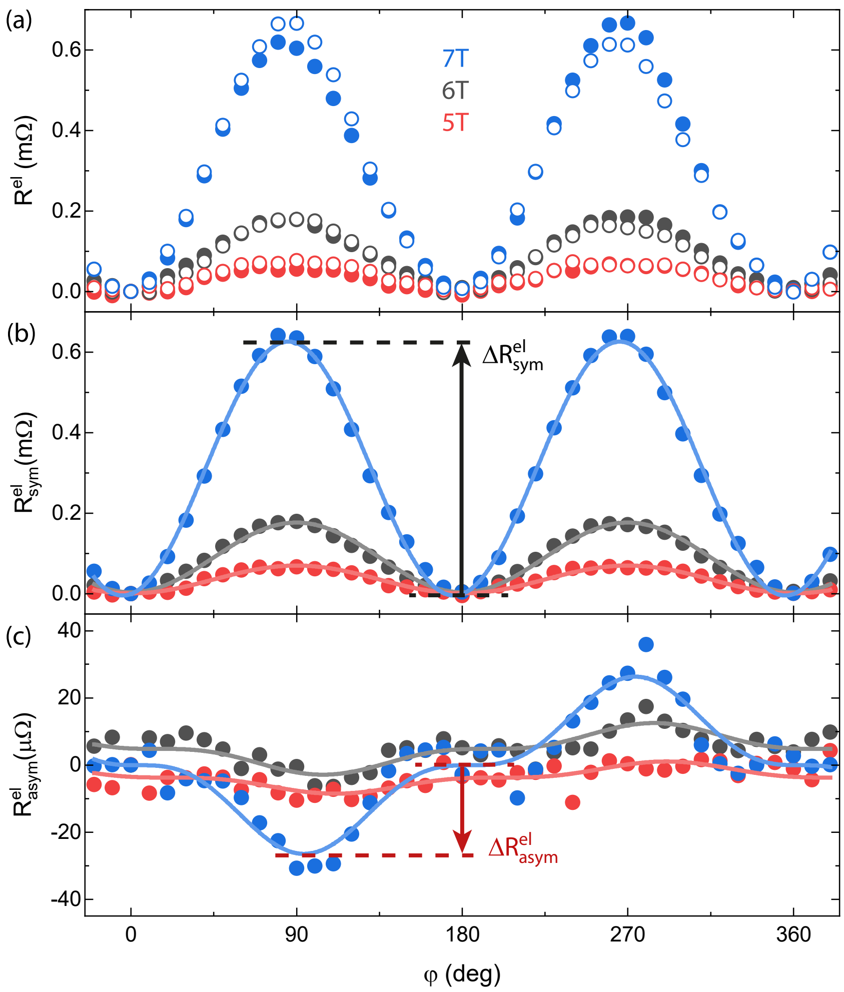


FIG. S2. (a) Angle-dependent magnon spin signal $R^{\mathrm{el}}$ for diffusive transport of magnons measured at $T = 200\,\mathrm{K}$ for a center-to-center electrode distance of $d = 0.75\,\mu\mathrm{m}$ and different magnetic field magnitudes for the 19 nm thin hematite film. The filled dots correspond to an injection of magnons at the left electrode and a detection of $R^{\mathrm{el}}$ at the right electrode, while the open circles correspond to the reversed measurement scheme as indicated in Fig. 2(a) in the main text. Note that a constant offset arising from the experimental setup has been subtracted from the curves. (b) Symmetric part $R^{\mathrm{el}}_{\mathrm{sym}}$ of the two measurement configurations for the respective magnetic fields in panel (a). The lines are fits to a simple $\Delta R^{\mathrm{el}}_{\mathrm{sym}} \sin^2(\varphi)$ function, which is expected in the absence of an antisymmetric contribution. (c) Antisymmetric signal part $R^{\mathrm{el}}_{\mathrm{asym}}$ of the respective curves in panel (a). The lines represent a $\Delta R^{\mathrm{el}}_{\mathrm{asym}} \sin^3(\varphi)$ angular dependence.

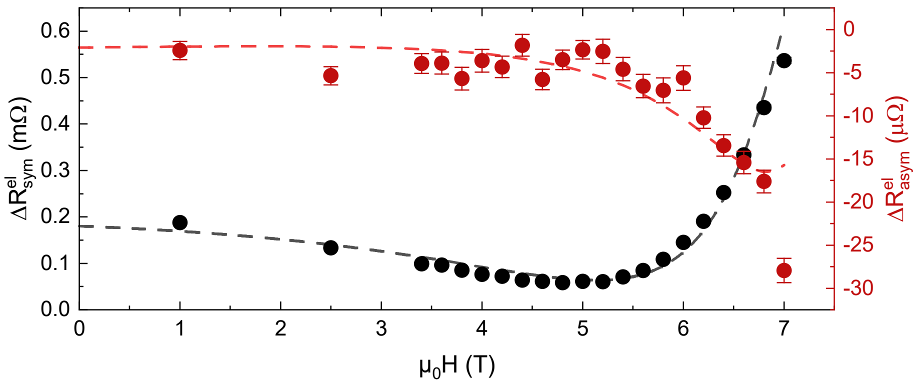


FIG. S3. Magnetic field-dependence of $\Delta R^{\mathrm{el}}_{\mathrm{sym}}$ (black dots) and $\Delta R^{\mathrm{el}}_{\mathrm{asym}}$ (red dots) extracted from Fig. S2. The dashed lines are fits to Eq. (2) in the main text. For the $t_{\mathrm{m}} = 19\,\mathrm{nm}$ thin film we are limited to the $\omega < 0$ configuration and thus observe no sign change in $\Delta R^{\mathrm{el}}_{\mathrm{asym}}$.

| Symbol | Unit | $Fe_2O_3$(19 nm) | $Fe_2O_3$(89 nm) |
|---|---|---|---|
| $d$ | µm | 0.75 | 1.2 |
| $D_{\mathrm{m}}$ | $10^{-4}\mathrm{m}^2/\mathrm{s}$ | $1.6 \pm 0.7$ | $1.8 \pm 1.3$ |
| $\tau_{\mathrm{m}}$ | $10^{-9}\mathrm{s}$ | $1.2 \pm 0.3$ | $0.8 \pm 0.2$ |
| $c_1$ | $10^{9}\mathrm{s}^{-1}$ | $8.0 \pm 2.3$ | $6.0 \pm 4.0$ |
| $c_2$ | $10^{9}\mathrm{m}/(\mathrm{As})$ | $1.1 \pm 0.3$ | $1.0 \pm 0.6$ |
| $A$ | $\Omega\mathrm{m}/\mathrm{s}$ | $1.3 \pm 0.1$ | $17.2 \pm 3.5$ |
| $R^0_{\mathrm{sym}}$ | mΩ | $0.19 \pm 0.01$ | $2.2 \pm 0.1$ |
| $\delta\omega l$ | m/s | $-9.9 \pm 1.4$ | $-11.2 \pm 0.7$ |
| $R^0_{\mathrm{asym}}$ | µΩ | $-2.6 \pm 1.0$ | $-8.9 \pm 2.7$ |

TABLE S1. Device dependent parameters extracted from fits to Eqs. (S2) and (S3) in Fig. S3 and Fig. (3) in the main text.

For a quantitative explanation, we extract the amplitudes $\Delta R^{\mathrm{el}}_{\mathrm{sym}}$ and $\Delta R^{\mathrm{el}}_{\mathrm{asym}}$ from the fits in Fig. S2 and plot them as a function of the magnetic field magnitude $\mu_0 H$ in Fig. S3. The amplitude of the symmetric part exhibits a rather constant behavior $\Delta R^{\mathrm{el}}_{\mathrm{sym}} = 0.1\,\mathrm{m}\Omega$ between $\mu_0 H = 1\,\mathrm{T}$ and $6\,\mathrm{T}$, while it significantly increases for $\mu_0 H > 6\,\mathrm{T}$. We can attribute this behavior to the onset of the Hanle peak and hence can describe the data with $\mu_{\mathrm{sym}}$, which is fitted to the data (gray dashed line). Note that we do not reach the compensation field $\mu_0 H_{\mathrm{c}}$ within the limits of our setup and therefore $\omega < 0$ over the whole magnetic field

range. We observe a similar field-dependent behavior for the antisymmetric contribution with $\Delta R^{\mathrm{el}}_{\mathrm{asym}} \approx -5\,\mu\Omega$ between $\mu_0 H = 1\,\mathrm{T}$ and $6\,\mathrm{T}$ and a strongly enhanced negative signal $\Delta R^{\mathrm{el}}_{\mathrm{asym}}$ for $\mu_0 H > 6\,\mathrm{T}$. We can describe the behavior via $\mu_{\mathrm{asym}}$ defined in Eq. (2) in the main text. Analogue to our previous work [S2], we treat the pseudofield $\boldsymbol{\omega}$ as an experimentally observed field for the studied easy-plane hematite film and express the precession frequency as $\omega = c_2 H - c1$ after performing a Taylor expansion of $\omega$ around $H_{\mathrm{c}}$. Note that the physical meaning of $c_1$ and $c_2$ is dependent on the microscopic origin of the pseudofield. In a first step, we fitted the symmetric signal $\Delta R^{\mathrm{el}}_{\mathrm{sym}}$ employing the following function:

$$\Delta R^{\mathrm{el}}_{\mathrm{sym}} = R^{0}_{\mathrm{sym}} + \frac{A l_{\mathrm{m}} e^{-\frac{ad}{l_{\mathrm{m}}}}}{D_{\mathrm{m}}\left(a^2+b^2\right)} \left[ a\cos\left(\frac{bd}{l_{\mathrm{m}}}\right) - b\sin\left(\frac{bd}{l_{\mathrm{m}}}\right) \right], \tag{S2}$$

where $a \equiv \sqrt{\left(1+\sqrt{1+\omega^2\tau_{\mathrm{m}}^2}\right)/2}$, $b \equiv \sqrt{\left(-1+\sqrt{1+\omega^2\tau_{\mathrm{m}}^2}\right)/2}$, and $l_m \equiv \sqrt{D_{\mathrm{m}}\tau_{\mathrm{m}}}$ analog to the main text. As free parameters we choose $D_{\mathrm{m}}$, $\tau_{\mathrm{m}}$, $c_1$, $c_2$, $A$ and $R^{0}_{\mathrm{sym}}$, while the center-to-center distance $d$ is given by the geometry of the device and is fixed. While $A = A_0 j_{\mathrm{s0}}/\chi$, where $A_0$ acts as a constant scaling parameter to take into account the conversion effects from the pseudospin chemical potential to the measured detector signal $\Delta R^{\mathrm{el}}_{\mathrm{sym}}$, $R^{0}_{\mathrm{sym}}$ accounts for a finite offset.

In a second step, we fitted the antisymmetric signal $\Delta R^{\mathrm{el}}_{\mathrm{asym}}$. The fitting function reads

$$\begin{aligned} \Delta R^{\mathrm{el}}_{\mathrm{asym}} = R^{0}_{\mathrm{asym}} + \frac{\omega\delta\,\omega\,\tau_{\mathrm{m}} l}{|\omega| 2 l_{\mathrm{m}}} \Bigg[ & -\frac{2 A l_{\mathrm{m}} b e^{-\frac{ad}{l_{\mathrm{m}}}} \left( a\cos\left(\frac{bd}{l_{\mathrm{m}}}\right) - b\sin\left(\frac{bd}{l_{\mathrm{m}}}\right)\right)}{D_{\mathrm{m}}(a^2+b^2)^2} \\ & + \frac{A l_{\mathrm{m}} e^{-\frac{ad}{l_{\mathrm{m}}}} \left( -\frac{bd}{l_{\mathrm{m}}}\cos\left(\frac{bd}{l_{\mathrm{m}}}\right) - \sin\left(\frac{bd}{l_{\mathrm{m}}}\right) - \frac{ad}{l_{\mathrm{m}}}\sin\left(\frac{bd}{l_{\mathrm{m}}}\right)\right)}{D_{\mathrm{m}}(a^2+b^2)} \Bigg]. \end{aligned} \tag{S3}$$

We utilize the extracted parameters from the symmetric contribution as fixed parameters, only leaving $\delta\omega l$ as a free fit parameter. Furthermore, we allowed for an additional offset signal $R^{0}_{\mathrm{asym}}$. The theory curve (red dashed line) reproduces $\Delta R^{\mathrm{el}}_{\mathrm{asym}}$ well in the low magnetic field regime, however we find a difference around $\mu_0 H = 7\,\mathrm{T}$. While the antisymmetric signal significantly increases, the theory curve suggests a decrease of the signal. This might be caused by uncertainties in the fitting procedure as we are limited to $\mu_0 H = 7\,\mathrm{T}$ and hence can only fit the onset of the Hanle curve instead of the full peak. The same fit procedure has been employed for the 89 nm thick hematite layer presented in the main text in Fig. 3. The extracted fit parameters for both films can be found in Tab. S1.

Furthermore, we find that $\Delta R^{\mathrm{el}}_{\mathrm{sym}}$ is about one order of magnitude smaller compared to the thicker hematite film investigated in the main text. However, the antisymmetric signal $\Delta R^{\mathrm{el}}_{\mathrm{asym}}$ exhibits the same order of magnitude for both film thicknesses. For the 19 nm thin film, measurements at higher magnetic field magnitudes are needed to verify the expected sign change in $\Delta R^{\mathrm{el}}_{\mathrm{asym}}$ at the compensation field of the Hanle curve that we demonstrated for the thicker film in the main text.


[S1] F. J. Morin, Magnetic susceptibility of $\alpha - Fe_2O_3$ and $\alpha - Fe_2O_3$ with added titanium, Phys. Rev. **78**, 819 (1950).

[S2] J. Gückelhorn, A. Kamra, T. Wimmer, M. Opel, S. Geprägs, R. Gross, H. Huebl, and M. Althammer, Influence of low-energy magnons on magnon hanle experiments in easy-plane antiferromagnets, Phys. Rev. B **105**, 094440 (2022).

[S3] T. Wimmer, A. Kamra, J. Gückelhorn, M. Opel, S. Geprägs, R. Gross, H. Huebl, and M. Althammer, Observation of antiferromagnetic magnon pseudospin dynamics and the hanle effect, Phys. Rev. Lett. **125**, 247204 (2020).
